# Supplementary material for: Preconditioned quantum linear system algorithm
Source: arXiv:1301.2340 ancillary file (2013-05-07)
Supplement: Supplementary file 1 [file qlsa_supplementary.pdf]

# Preconditioned quantum linear system algorithm: supplementary material

B. D. Clader, B. C. Jacobs, and C. R. Sprouce
*The Johns Hopkins University Applied Physics Laboratory, Laurel, MD 20723*

## I. INTRODUCTION

In this supplementary material, we present many of the specific details behind the theory of the quantum linear systems algorithm (QLSA) [1], and we present our deterministic version of the algorithm that fully incorporates amplitude estimation (AE) [2] into the original algorithm and the measurement process. To aid the reader's understanding of the scattering cross section application of our algorithm, we present the quantum oracles required to implement the algorithm. These oracles solve a simple toy scattering problem, on a two-dimensional square grid with first order absorbing boundary conditions. We note that our algorithm can be generalized to three-dimensional problems on non-square grids with higher order boundary conditions and non-metallic scatterers. We chose the simple scattering problem, simply as an example.

## II. QUANTUM ALGORITHM IMPLEMENTATION

The QLSA determines the solution to

$$A|x\rangle = |b\rangle, \tag{1}$$

where $A$ is an $N \times N$ sparse matrix, and $b$ is an $N \times 1$ vector of known values. To improve convergence properties we instead solve the preconditioned linear system

$$MA|x\rangle = M|b\rangle \qquad \text{or} \qquad AM|y\rangle = |b\rangle, \tag{2}$$

where $|y\rangle = M^{-1}|x\rangle$. These are denoted as left and right preconditioning methods respectively, and the matrix $M$ is referred to as the matrix preconditioner One gains if the matrix $A' = MA$ (or $A' = AM$) has a reduced condition number relative to $A$ causing preconditioned linear system solvers to have faster convergence than un-preconditioned cases. If one maps $MA \to A$ and $M|b\rangle \to |b\rangle$ (or $AM \to A$ and $|y\rangle \to |x\rangle$), then the quantum portion of the algorithm for both preconditioned and non-preconditioned cases are identical. Therefore in this supplementary material, which is included as an aid to understanding the details of the quantum algorithm, we proceed as if we are solving Eq. (1) without any loss of generality.

For non-Hermitian $A$ matrices, we follow the reduction outlined in [1] which restates the variables $A$, $|b\rangle$ and $|x\rangle$ as

$$\bar{A} = \begin{pmatrix} 0 & A \\ A^\dagger & 0 \end{pmatrix}, \qquad |\bar{b}\rangle = \begin{pmatrix} |b\rangle \\ 0 \end{pmatrix}, \qquad \text{and} \qquad |\bar{x}\rangle = \begin{pmatrix} 0 \\ |x\rangle \end{pmatrix}, \tag{3}$$

where the 0 entries are 0 amplitude vectors the same length as $|x\rangle$ and $|b\rangle$. With this redefinition, we simply solve $\bar{A}|\bar{x}\rangle = |\bar{b}\rangle$. The solution will now be stored in a vector of length $2N$ where the first $N$ amplitudes are 0. The rest of the QLSA proof will proceed assuming this redefinition and taking $N \to 2N$.

Classical linear-system solvers can contain non-normalized "state"-vectors, which allow one to carry units. Of course in a quantum implementation all state vectors must be normalized. Since we wish to compute an actual physical quantity we must be able to restore units to the normalized solution. To avoid ambiguity, from here on any state vector will be assumed to be normalized, unless explicitly stated otherwise. At the termination of our algorithms results must be scaled appropriately.

To begin, prepare three quantum registers with the following states:

$$|\Psi\rangle = |\psi_1\rangle_1 |b_T\rangle_{2,6} \tag{4}$$

where register 1 contains

$$|\psi_1\rangle_1 = \frac{1}{\sqrt{T}} \sum_{\tau=0}^{T-1} |\tau\rangle_1 \tag{5}$$

and the state $|b_T\rangle_{2,6}$ is

$$|b_T\rangle_{2,6} = \cos\phi_b|\tilde{b}\rangle_2|0\rangle_6 + \sin\phi_b|b\rangle_2|1\rangle_6. \tag{6}$$

This is an entangled state, with the state needed for the solution of (1), contained in register 2 and entangled with the 1 value of qubit 6. The states $|b\rangle$ and $|\tilde{b}\rangle$ can be written in the computational basis as

$$|b\rangle = \frac{1}{\sqrt{N}\sin\phi_b}\sum_{j=0}^{N-1} C_b b_j e^{i\phi_j^{(b)}}|j\rangle \qquad |\tilde{b}\rangle = \frac{1}{\sqrt{N}\cos\phi_b}\sum_{j=0}^{N-1}\sqrt{1-C_b^2 b_j^2}e^{i\phi_j^{(b)}}|j\rangle, \tag{7}$$

where $b_j e^{i\phi_j^{(b)}}$ are the individual complex terms contained in the vector $|b\rangle$. The oracle used to compute the elements is given in Eq. (77). The normalization factor is

$$\sin^2\phi_b = \frac{C_b^2}{N}\sum_{j=0}^{N-1} b_j^2 \qquad \cos^2\phi_b = \frac{1}{N}\sum_{j=0}^{N-1}(1-C_b^2 b_j^2), \tag{8}$$

and $C_b \leq 1/\max(b_j)$ to ensure all rotations are less than $2\pi$. Note here that the individual $b_j$ terms need not be normalized and can contain units, since they are divided by the maximum value. An efficient method to prepare state (6) is given in section III A.

Next the following controlled unitary operator is applied to the second register, controlled off the value in register 1:

$$U_{1,2} = \left(e^{iA\tau t_0/T}\right)_2, \tag{9}$$

The constant $t_0 = ||A||\kappa/\epsilon$ is chosen to minimize the error $\epsilon$ for a given condition number $\kappa$ and matrix norm $||A||$. This unitary operation is equivalent to a Hamiltonian simulation. It is here we see directly the impact of the condition number of $A$ on the time complexity of the algorithm, since the time complexity of Hamiltonian simulation scales at best linearly with the time needed for simulation [3].

After application of this controlled operation and expanding the state $|b\rangle_2 = \sum_{j=0}^{N-1}\beta_j|u_j\rangle_2$ and $|\tilde{b}\rangle_2 = \sum_{j=0}^{N-1}\tilde{\beta}_j|u_j\rangle_2$ into normalized eigenstates of the operator $A$, the state is in the following form

$$|\Psi\rangle \rightarrow \frac{1}{\sqrt{T}}\sum_{j=0}^{N-1}\sum_{\tau=0}^{T-1}\left(\cos\phi_b\tilde{\beta}_j e^{i\lambda_j\tau t_0/T}|\tau\rangle_1|u_j\rangle_2|0\rangle_6 + \sin\phi_b\beta_j e^{i\lambda_j\tau t_0/T}|\tau\rangle_1|u_j\rangle_2|1\rangle_6\right). \tag{10}$$

Next we apply the quantum Fourier transform to register 1 yielding the state

$$|\Psi\rangle \rightarrow \sum_{\tilde{\tau}=0}^{T-1}\sum_{j=0}^{N-1}\left(\cos\phi_b\tilde{\beta}_j\alpha_{\tilde{\tau}}|\tilde{\tau}\rangle_1|u_j\rangle_2|0\rangle_6 + \sin\phi_b\beta_j\alpha_{\tilde{\tau}}|\tilde{\tau}\rangle_1|u_j\rangle_2|1\rangle_6\right), \tag{11}$$

where

$$\alpha_{\tilde{\tau}} = \sum_{\tau=0}^{T-1}\frac{1}{T}\exp\left[-2\pi i\left(\tilde{\tau}-\frac{\lambda_j t_0}{2\pi}\right)\frac{\tau}{T}\right]. \tag{12}$$

The term $\alpha_{\tilde{\tau}}$ is a strongly peaked function about $\tilde{\tau} = \frac{\lambda_j t_0}{2\pi}$ (exactly a Kronicker delta if one had infinite bit precision). For simplicity we will assume that we have infinite precision, allowing for the delta function reduction. In general it is not true, and the full error analysis can be found in Ref. [1] and references therein. Assuming a delta function Eq. (11) becomes

$$|\Psi\rangle = \sum_{j=0}^{N-1}\left(\cos\phi_b\tilde{\beta}_j|\tilde{\lambda_j}\rangle_1|u_j\rangle_2|0\rangle_6 + \sin\phi_b\beta_j|\tilde{\lambda_j}\rangle_1|u_j\rangle_2|1\rangle_6\right), \tag{13}$$

where $\tilde{\lambda_j} = \lambda_j t_0/2\pi$. We now apply a rotation to register 6, conditioned on the bit value of register 1, leading to the state

$$|\Psi\rangle \rightarrow \sum_{j=0}^{N-1}\left(\cos\phi_b\tilde{\beta}_j|\tilde{\lambda_j}\rangle_1|u_j\rangle_2|0\rangle_6 + \sin\phi_b\beta_j|\tilde{\lambda_j}\rangle_1|u_j\rangle_2|1\rangle_6\right)\left(\sqrt{1-\frac{C^2}{\lambda_j^2}}|0\rangle_7 + \frac{C}{\lambda_j}|1\rangle_7\right), \tag{14}$$

where $C = 1/\kappa$ is a constant chosen such that each term $C/\lambda_j < 1$ since $\kappa = \lambda_{\max}/\lambda_{\min}$ (definition of the spectral condition number). We now reverse steps (10) and (11) to uncompute register 1 giving

$$|\Psi\rangle \rightarrow |0\rangle_1 \sum_{j=0}^{N-1} \left(\cos\phi_b \tilde{\beta}_j |u_j\rangle_2 |0\rangle_6 + \sin\phi_b \beta_j |u_j\rangle_2 |1\rangle_6\right) \left(\cos\theta_j |0\rangle_7 + \sin\theta_j |1\rangle_7\right), \tag{15}$$

where $\sin\theta_j = C/\lambda_j$ and $\cos\theta_j = \sqrt{1 - C^2/\lambda_j^2}$. For notational simplicity we will now collect all terms except for those entangled with $|1\rangle_6 |1\rangle_7$ into a state which we will call simply $|\Phi_0\rangle$. This allows us to rewrite Eq. (15) as

$$|\Psi\rangle = (1 - \sin^2\phi_b \sin^2\phi_x)^{1/2} |\Phi_0\rangle_{2,6,7} + \sin\phi_b \sin\phi_x |x\rangle_2 |1\rangle_6 |1\rangle_7, \tag{16}$$

where

$$|x\rangle = \frac{1}{\sin\phi_x} \sum_{j=0}^{N-1} \frac{C\beta_j}{\lambda_j} |u_j\rangle \tag{17}$$

is a normalized solution to $A|x\rangle = |b\rangle$ and $\sin^2\phi_x = C^2 \sum_{j=0}^{N-1} |\beta_j|^2/\lambda_j^2$.

Next we prepare the state

$$|R_T\rangle_{3,8} = \cos\phi_r |\tilde{R}\rangle_3 |0\rangle_8 + \sin\phi_r |R\rangle_3 |1\rangle_8 \tag{18}$$

using the same method we used to prepare the state $|b_T\rangle$. The states $|R\rangle$ and $|\tilde{R}\rangle$ can be written in the computational basis as

$$|R\rangle = \frac{1}{\sqrt{N}\sin\phi_r} \sum_{j=0}^{N-1} C_r r_j e^{i\phi_j^{(r)}} |j\rangle \qquad |\tilde{R}\rangle = \frac{1}{\sqrt{N}\cos\phi_r} \sum_{j=0}^{N-1} \sqrt{1 - C_r^2 r_j^2} e^{i\phi_j^{(r)}} |j\rangle, \tag{19}$$

where $r_j e^{i\phi_j^{(r)}}$ are the individual complex terms contained in the vector $|R\rangle$,

$$\sin^2\phi_r = \frac{C_r^2}{N} \sum_{j=0}^{N-1} r_j^2 \qquad \cos^2\phi_r = \frac{1}{N} \sum_{j=0}^{N-1} (1 - C_r^2 r_j^2), \tag{20}$$

and $C_r \leq 1/\max(r_j)$.

We now write the composite state from Eqs. (16) and (18) along with an adjoined ancilla qubit initialized to 0 as

$$|\Psi\rangle = (1 - \sin^2\phi_t)^{1/2} |\Phi_1\rangle_{2,3,6,7,8} |0\rangle_9 + \sin\phi_t |x\rangle_2 |R\rangle_3 |1\rangle_6 |1\rangle_7 |1\rangle_8 |0\rangle_9, \tag{21}$$

where $\sin\phi_t = \sin\phi_b \sin\phi_x \sin\phi_r$ and $|\Phi_1\rangle_{2,3,6,7,8}$ is the composite state of all seven other product terms in which qubits 6,7, and 8 are not all simultaneously 1.

A Hadamard transform is applied to the ancilla qubit 9 and a controlled swap operation is applied to registers 2 and 3 controlled on the value of the ancilla qubit 9 being a 1, followed by a second Hadamard on the ancilla. This gives

$$\begin{aligned} |\Psi\rangle \rightarrow\ & (1 - \sin^2\phi_t)^{1/2} |\Phi_2\rangle_{2,3,6,7,8,9} \\ & + \frac{1}{2}\sin\phi_t [(|x\rangle_2 |R\rangle_3 + |R\rangle_2 |x\rangle_3)|0\rangle_9 + (|x\rangle_2 |R\rangle_3 - |R\rangle_2 |x\rangle_3)|1\rangle_9] |1\rangle_6 |1\rangle_7 |1\rangle_8, \end{aligned} \tag{22}$$

where $|\Phi_2\rangle_{2,3,6,7,8,9}$ is a composite state, resulting from this sequence of operations, containing all fourteen terms where qubits 6,7, and 8 are not 1. Next we expand the state $|x\rangle = x_r |R\rangle + x_\perp |R_\perp\rangle$ into the components parallel and perpendicular to the state $|R\rangle$. In doing so, Eq. (22) becomes

$$\begin{aligned} |\Psi\rangle \rightarrow\ & (1 - \sin^2\phi_t)^{1/2} |\Phi_2\rangle_{2,3,6,7,8,9} \\ & + \frac{1}{2}\sin\phi_t \big[2x_r |R\rangle_2 |R\rangle_3 + x_\perp (|R\rangle_2 |R_\perp\rangle_3 + |R_\perp\rangle_2 |R\rangle_3)\big] |1\rangle_6 |1\rangle_7 |1\rangle_8 |0\rangle_9 \\ & + \frac{1}{2}\sin\phi_t x_\perp \big(|R_\perp\rangle_2 |R\rangle_3 - |R\rangle_2 |R_\perp\rangle_3\big) |1\rangle_6 |1\rangle_7 |1\rangle_8 |1\rangle_9. \end{aligned} \tag{23}$$

Thus the probability of measuring a 1 in qubits 6-9 is given by $P_{1111} = \sin^2\phi_t |x_\perp|^2/2$, while the probability to measure a 1 in qubits 6-8 and a 0 in qubit 9 is $P_{1110} = \sin^2\phi_t(|x_r|^2 + |x_\perp|^2/2)$. The dot product between $|R\rangle$ and $|x\rangle$ can be written in terms of these probabilities as

$$|\langle R|x\rangle|^2 = |x_r|^2 = \frac{1}{\sin^2\phi_t}(P_{1110} - P_{1111}), \tag{24}$$

where $P_{1110}$ and $P_{1111}$ refer to the probability of measuring a 1 in register 6-7 and a 0 or 1 in qubit 8 respectively. These quantities can be estimated deterministically with error $\epsilon$ using amplitude estimation [2].

The final step is to now restore units to the normalized states $|R\rangle$ and $|x\rangle$. To do so we go back to their original definitions in Eqs. (17) and (19) and compute

$$|\langle R|x\rangle|^2 = \frac{C_r^2}{N\sin^2\phi_r}\left|\sum_{j=0}^{N-1} r_j e^{-i\phi_j^{(r)}} x_j^{(n)}\right|^2, \tag{25}$$

where $x_j^{(n)}$ is the normalized amplitude of the state $|x\rangle$ in the computational basis. Next we multiply $|x\rangle$ by the normalization constant for state $|b\rangle$ which is $\sqrt{N}\sin\phi_b/C_b$ and divide by the probability that the QLSA produces the state $|x\rangle$ from the state $|b\rangle$, which is $\sin\phi_x$, giving

$$\frac{N\sin^2\phi_b}{C_b^2\sin^2\phi_x}|\langle R|x\rangle|^2 = \frac{C_r^2}{N\sin^2\phi_r}\left|\sum_{j=0}^{N-1} r_j e^{-i\phi_j^{(r)}} x_j\right|^2, \tag{26}$$

where $x_j = [\sqrt{N}\sin\phi_b/(C_b\sin\phi_x)]x_j^{(n)}$ is the amplitude of the state $|x\rangle$ in units of the $b_j$ terms. Combining Eqs. (24) and (26) gives

$$\left|\sum_{j=0}^{N-1} r_j e^{-i\phi_j^{(r)}} x_j\right|^2 = \frac{N^2\sin^2\phi_b\sin^2\phi_r}{C_b^2C_r^2\sin^2\phi_x}(P_{1110} - P_{1111}). \tag{27}$$

Thus the dot product of the un-normalized vector $|R_u\rangle = \sum_{j=0}^{N-1} r_j e^{i\phi_j^{(r)}}|j\rangle$ with the un-normalized vector $|x_u\rangle = A^{-1}|b_u\rangle$ can be calculated, allowing one to restore desired units after running the quantum algorithm. Finally, to aid in understanding the computational procedure that we envision, a flowchart demonstrating how all the various components we have mentioned fit together is shown in Fig. 1.

## III. QLSA SUBROUTINES

The QLSA requires many routines that were mentioned but not fully explained in the previous section. These are state preparation, amplitude estimation, and phase estimation. In this section, we will describe these subroutines in more detail. Phase estimation requires Hamiltonian simulation and a quantum Fourier transform (QFT). Since the QFT is trivial, we will focus on the Hamiltonian simulation algorithm in this section.

### A. State Preparation

The QLSA requires that quantum registers be prepared in arbitrary states $|b\rangle$ and $|R\rangle$. Here we will use notation denoting the preparation of state $|b\rangle$, and simply note that this applies equally well to any state, including $|R\rangle$. Efficiently preparing an arbitrary state is an open area of interest [4–8], and is not necessarily possible for general cases. However it is possible to prepare the following state

$$|b_T\rangle_{2,6} = \cos\phi_b|\tilde{b}\rangle_2|0\rangle_6 + \sin\phi_b|b\rangle_2|1\rangle_6, \tag{28}$$

where register 2 contains the desired arbitrary state $|b\rangle$ entangled with a 1 in register 6, or a "junk" state $|\tilde{b}\rangle$ entangled with a 0 in register 6. See Eq. (7) for more details. Preparation of (28) is efficient so long as an oracle exists that can efficiently compute the amplitudes of $|b\rangle$. For clarity, we note here that one is preparing the preconditioned state

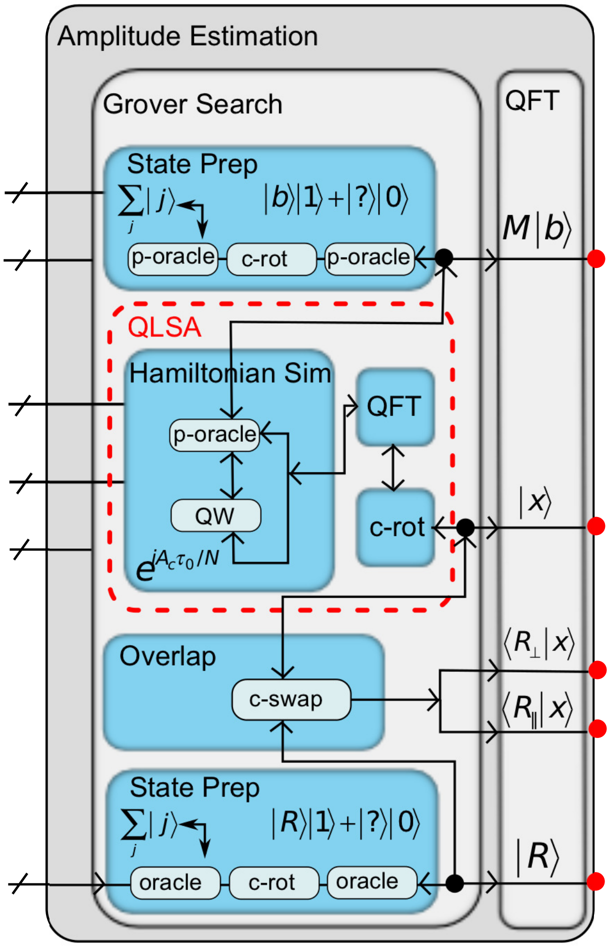


FIG. 1. Flowchart describing the envisioned operation of the quantum algorithm. Wires denote quantum registers, various subroutines are shown in the blue boxes, operations in light blue boxes, and measurements are denoted by red dots. The entire algorithm is contained within an amplitude estimation routine that itself consists of a controlled Grover search, and a quantum Fourier transform (QFT). After state preparation of both $|b\rangle$ and $|R\rangle$ states, AE is used to determine $\sin^2\phi_b$ and $\sin^2\phi_r$. These are the top and bottom measurements. After the QLSA algorithm AE is used to estimate $\sin^2\phi_x$. Finally, after the entire algorithm is run, including the controlled swap operation, the overlap integrals are calculated with amplitude estimation. All measurements are combined using Eq. (24) to produce an estimate of the overlap integral. The denoted "p-oracle" indicates where the preconditioning step is integrated with the oracles to produce the preconditioned linear system.

$M|b\rangle$. However, one sees that this enters through the oracle used to compute the elements of $|b\rangle$. We will describe how this is done later in the paper.

To prepare state $|b_T\rangle$ this we initialize registers 2,4-6 as

$$|\Psi\rangle = \frac{1}{\sqrt{N}}\sum_{j=0}^{N-1}|j\rangle_2|0\rangle_4|0\rangle_5|0\rangle_6. \tag{29}$$

An oracle is queried that calculates the $b_j$ and $\phi_j$ coefficients. This operation is controlled off of the index value stored in register 2. This results in the state

$$|\Psi\rangle \rightarrow \frac{1}{\sqrt{N}}\sum_{j=0}^{N-1}|j\rangle_2|b_j\rangle_4|\phi_j\rangle_5|0\rangle_6. \tag{30}$$

Next, apply a controlled phase gate to the ancilla qubit in register 6, controlled by the value stored in register 5. The circuit to apply the controlled phase is shown in Fig. 6. This gives

$$|\Psi\rangle \to \frac{1}{\sqrt{N}} \sum_{j=0}^{N-1} e^{i\phi_j} |j\rangle_2 |b_j\rangle_4 |\phi_j\rangle_5 |0\rangle_6. \tag{31}$$

We now rotate register 6 conditioned on the value contained in register 4, and uncompute registers 4 and 5 by simply calling the $b_j$ and $\phi_j$ oracles again leaving

$$|\Psi\rangle \to \frac{1}{\sqrt{N}} \sum_{j=0}^{N-1} e^{i\phi_j} |j\rangle_2 |0\rangle_4 |0\rangle_5 \left( \sqrt{1 - C_b^2 b_j^2} |0\rangle_6 + C_b b_j |1\rangle_6 \right), \tag{32}$$

where $C_b \le 1/\max(b_j)$ to ensure that all rotations are less than $2\pi$. State (32) is now exactly the state (28) with the definitions of $\cos^2\phi_b$ and $\sin^2\phi_b$ given in (8). This state preparation algorithm is efficient as long as the unitary operator used to compute $b_j$ and $\phi_j$ is efficient.

### B. Amplitude Estimation

For a general case, state preparation could be accomplished by simply measuring the ancilla qubit in (32) and only accepting the results when the ancilla is 1. For the QLSA we can avoid this probabilistic process, and replace it with amplitude estimation [2] that we use to estimate the weighting coefficients. Throughout our implementation of QLSA we will repeatedly apply this technique to multiple ancilla in order to avoid nested non-deterministic routines.

For a general case suppose we have a unitary operator $U$ that operates on the $|0\rangle_m$ state giving

$$U|0\rangle_m = \cos\phi |\Phi_0\rangle_m + \sin\phi |\Phi_1\rangle_m, \tag{33}$$

where the register labelled $m$ contains an arbitrary number of qubits, and the states $|\Phi_0\rangle$ and $|\Phi_1\rangle$ are arbitrary. The goal of amplitude estimation is to estimate $a \equiv \sin^2\phi$ to within $\pm\epsilon a$ accuracy. To do so, we define the following operator

$$Q = U(2|0\rangle\langle 0| - 1)U^\dagger S_\chi, \tag{34}$$

where $S_\chi$ is the Grover oracle and operates as

$$\begin{aligned} S_\chi |\Phi_0\rangle_m &= |\Phi_0\rangle_m \\ S_\chi |\Phi_1\rangle_m &= -|\Phi_1\rangle_m. \end{aligned} \tag{35}$$

It is straightforward to show that $Q$ has the following action on the state $U|0\rangle_m$

$$\begin{aligned} Q^j U|0\rangle_m &= Q^j \left(\cos\phi |\Phi_0\rangle_m + \sin\phi |\Phi_1\rangle_m\right) \\ &= \cos\left[(2j+1)\phi\right] |\Phi_0\rangle_m + \sin\left[(2j+1)\phi\right] |\Phi_1\rangle_m. \end{aligned} \tag{36}$$

The AE algorithm now proceeds as follows. Initialize a state to

$$|\Psi\rangle \to \frac{1}{\sqrt{M}} \sum_{j=0}^{M-1} |j\rangle_0 |0\rangle_m. \tag{37}$$

Next, apply the $U$ operator (33) giving the state

$$|\Psi\rangle \to= \frac{1}{\sqrt{M}} \sum_{j=0}^{M-1} |j\rangle_0 (\cos\phi |\Phi_0\rangle_m + \sin\phi |\Phi_1\rangle_m), \tag{38}$$

followed by the $Q^j$ operator (34) controlled on the value $|j\rangle_0$

$$|\Psi\rangle \to= \frac{1}{\sqrt{M}} \sum_{j=0}^{M-1} |j\rangle_0 \big\{ \cos\left[(2j+1)\phi\right] |\Phi_0\rangle_m + \sin\left[(2j+1)\phi\right] |\Phi_1\rangle_m \big\}. \tag{39}$$

Finally, a Fourier transform is applied to register 0 yielding

$$|\Psi\rangle \to \frac{1}{2}\sum_{k=0}^{M-1}|k\rangle_0\left[\tilde{\alpha}_{-k}e^{i\phi}(|\Phi_0\rangle_m - i|\Phi_1\rangle_m) + \tilde{\alpha}_k e^{-i\phi}(|\Phi_0\rangle_m + i|\Phi_1\rangle_m)\right] \tag{40}$$

where

$$\tilde{\alpha}_{\mp k} = \frac{1}{M}\sum_{j=0}^{M-1} e^{2\pi i(k\pm M\phi/\pi)j/M} \tag{41}$$

is a sharply peaked function about $k = M\phi/\pi$ or $k = M - M\phi/\pi$. If we have infinite precision then Eq. (41) is exactly a Kronecker Delta function. Assuming this to be these case Eq. (40) becomes

$$\begin{aligned}|\Psi\rangle \to\ & \frac{1}{2}|k = M - M\phi/\pi\rangle_0 e^{i\phi}(|\Phi_0\rangle_m - i|\Phi_1\rangle_m) \\ &+ \frac{1}{2}|k = M\phi/\pi\rangle_0 e^{-i\phi}(|\Phi_0\rangle_m + i|\Phi_1\rangle_m).\end{aligned} \tag{42}$$

Thus, measuring register 0 and denoting the value by $y$ produces either $y = M - M\phi/\pi$ or $y = M\phi/\pi$. Since we are interested in the amplitude $a = \sin^2\phi$, we have as our estimate $a = \sin^2(\pi y/M)$ for both possible values of $y$. In reality, we will only have finite precision. Therefore Eq. (41) will not result in perfect delta functions. Thus in order to ensure that our estimate for $a$ is always within $\pm\epsilon a$ of the correct value we take $M = 2^{\lceil \log_2(1/\epsilon) + \log_2(\pi/(2\epsilon)+\pi)\rceil}$. More information on this error analysis can be found in [2].

### C. Hamiltonian Simulation

Hamiltonian Simulation is used by the QLSA during phase estimation. While the mathematical details of applying this unitary operator are straightforward, doing so efficiently on a quantum computer requires manipulation. In the worst case scenario such a unitary could require up to $O(N^2)$ gates to implement. Therefore even though the QLSA is exponentially faster than its classical counterpart, if an efficient way to apply $e^{-iAt}$ is not available, then the complexity is simply transferred to the gate level.

Here we will use the technique proposed by [3] to simulate sparse Hamiltonians and approximate the operator in Eq. (9). The approach is to decompose the operation into efficient components by breaking up the matrix $A = \sum_{j=1}^{m} A_j$ into $m$ sub-matrices, each of which are 1-sparse (maximum of 1 non-zero element per row and column), and where $m$ is at most $O(\log N)$. Each individual unitary is then applied as $e^{-iA_j t}$ in a specific manner such that they approximate the total operator $e^{-iAt}$.

The rest of section is organized as follows. Section III C 1 describes how to apply the 1-sparse sub-Hamiltonians such that they approximate the general Hamiltonian to within $\epsilon$ accuracy by using the Suzuki higher order integrator method. Section III C 3 describes how the actual decomposition is accomplished by using graph coloring techniques. In section III C 4 we provide the circuits necessary to apply the individual sub-Hamiltonians.

#### 1. *Suzuki Higher Order Integrators*

Since the individual $A_j$'s do not generally commute with each other we cannot simply apply them in succession, i.e. $U \neq \prod_{j=1}^{m} e^{-iA_j t}$. Instead we apply each $A_j$ according to the higher order integrator method of Suzuki [9]. In this case one can approximate the operator $e^{-iAt} \approx S_{2k}(-it) + O(|t|^{2k+1})$, where $S_{2k}(-it)$ is recursively defined as

$$S_{2k}(-it) \equiv \left[S_{2k-2}(-ip_k t)\right]^2 S_{2k-2}(-i(1-4p_k)t)\left[S_{2k-2}(-ip_k t)\right]^2 \tag{43}$$

with

$$S_2(-it) \equiv \prod_{j=1}^{m} e^{-iA_j t/2} \prod_{j'=m}^{1} e^{-iA_{j'} t/2}, \tag{44}$$

and $p_k \equiv (4 - 4^{1/(2k-1)})^{-1}$. Then

$$\left\| e^{-iAt} - S_{2k}(-it)\right\| = O(|t|^{2k+1}). \tag{45}$$

As a simple case, take $k = 1$, $m = 2$, and $r = 1$. Then $U = e^{-i(A_1+A_2)t} \approx S_2(-it) = e^{-iA_1t/2}e^{-iA_2t}e^{-iA_1t/2}$. This is the second order expansion of the Lie-Trotter formula $e^{A+B} = \lim_{n\to\infty}(e^{A/n}e^{B/n})^n$ [10]. The Suzuki higher order integrator method is then the generalization of the Lie-Trotter formula to order $k$ for $m$ operators.

To reduce the error in estimating the Hamiltonian by the sum of smaller Hamitonians, one divides the time into $r$ segments, then applies Eq. (43) $r$ times. Berry *et al.* [3] show that this error is bounded by

$$\left\| \exp\left(-it\sum_{j=1}^{m} A_j\right) - [S_{2k}(-it/r)]^r \right\| \le 2\left(2m5^{k-1}\|A\|\,t\right)^{2k+1}/r^{2k}, \tag{46}$$

where $\|A\|$ is the matrix norm. Under the requirement that the error is bounded by $\epsilon$ one sees that

$$r = \lceil 2^{1/2k}(2m5^{k-1}\|A\|t)^{1+\frac{1}{2k}}/\epsilon^{1/2k}\rceil. \tag{47}$$

Therefore, since the number of operators in $S_{2k}$ does not exceed $2m5^{k-1}$, one can show that the total number of exponential unitary operators required to approximate $e^{-iAt}$ to within $\epsilon$ is

$$N_{\rm exp} \le 2m5^{k-1}r = m^2 5^{2k}\|A\|t\left(\frac{m\|A\|t}{\epsilon}\right)^{1/2k}. \tag{48}$$

### *2. Hamiltonian Decomposition*

The preceding section shows how one can approximate the unitary operator given in Eq. (9) as

$$U \approx \left[S_{2k}\left(-\frac{it}{r}\right)\right]^r, \tag{49}$$

where $S_{2k}$ is a recursively defined function of simple unitary operators. Our goal now is to minimize the number of operations required to implement (49) by limiting the number of sub-matrices in our decomposition of $A$. Thus we wish to minimize $m$ in the decomposition $A = \sum_{j=1}^{m} A_j$ subject to the constraint that each $e^{-iA_jt}$ can be applied with an efficient quantum circuit.

Such an algorithm has been derived for arbitrary sparse matrices in Ref. 3. We will restate their technique here, using much of their original notation, and provide a simple example to illustrate it. The method decomposes the matrix as $A = \sum_{j=1}^{6d^2} A_j$, where $d$ is the maximum number of non-zero elements in a column of $A$. This method makes use of an oracle. The oracle $f(y,i)$ when queried with a row $y$ and an index $i$ will return $[A(y,x),x] = f(y,i)$, where $x$ is the column index corresponding to the $i^{th}$ non-zero element of the $y^{th}$ row. If $i$ is an invalid index, then the oracle returns $[0,i] = f(y,i)$. This oracle must be efficient, meaning that computation of these values does not scale with the size of the matrix. This method can decompose the matrix $A$ with $O(\log^* N)$ queries.

Consider the matrix $A$ as a graph, where the nodes are the rows of the graph, and the edges connecting these nodes to other nodes are the non-zero elements in that row. The edge connecting node $x$ to node $y$ will be called edge $(x,y)$. A simple $6\times 6$ example is shown in Fig. 2 where we take the matrix elements to be 1 for simplicity.

We color each edge by calling the oracle with $f(x,i) = [y, A(x,y)]$ and $f(y,j) = [x, A(y,x)]$. The edge is colored with the ordered pair $(i,j)$ if $y \ge x$, or $(j,i)$ if $x > y$. This is not generally a unique edge coloring since there exist long chains for which adjacent edges will be the same color. This first coloring step is shown in Fig. 3. This step takes exactly 2 queries to the oracle.

Next we eliminate the ambiguity in the previous edge coloring step, by including a third index for the edge such that each edge will be colored $(i,j,\nu)$. The determination of $\nu$ takes a maximum of $2(\log^* N+3)$ or $O(\log^* N)$ queries to implement, where $\log^* x = 1 + \log^*(\log_2 x)$ with $\log^* x = 0$ if $x < 1$ is the iterated logarithm. This coloring step makes use of the "deterministic coin tossing" algorithm [11, 12].

First, we set $x_0^{(0)} = x$ and determine the sequence of vertices that are connected to $x$ with color $(i,j)$:

$$x_0^{(0)} < x_1^{(0)} < x_2^{(0)} < \cdots \tag{50}$$

Usually chains consists of only two elements, however for some Hamiltonians long chains may be formed. In this case, the coloring algorithm only need sequence values up to vertex $\log^* N + 1$ to correctly edge color the graph, which for any realistic problem size will be 7 or less.

At the $0^{th}$ iteration each edge is labelled $(i,j,\nu)$ with the same $(i,j)$ for each edge. We begin by assigning $\nu$ the trivial solution, namely we color edge $(x_l, x_{l+1})$ with $x_l$. Next we update the sequence of values to $x_l^{(1)}$ in the following

$$A = \begin{pmatrix} 0 & 1 & 0 & 0 & 0 & 0 \\ 1 & 0 & 1 & 1 & 0 & 0 \\ 0 & 1 & 0 & 0 & 0 & 0 \\ 0 & 1 & 0 & 0 & 1 & 1 \\ 0 & 0 & 0 & 1 & 0 & 1 \\ 0 & 0 & 0 & 1 & 1 & 0 \end{pmatrix}$$

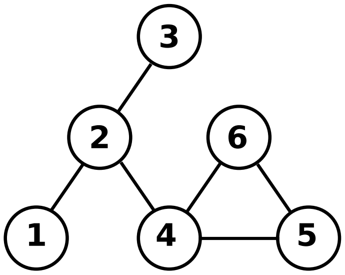


FIG. 2. The matrix on the left can be represented by the graph on the right. The matrix rows and column numbers are given by the vertices of the graph, while the edges correspond to the non-zero elements of the matrix.

$$A = \begin{pmatrix} 0 & 1 & 0 & 0 & 0 & 0 \\ 1 & 0 & 0 & 0 & 0 & 0 \\ 0 & 0 & 0 & 0 & 0 & 0 \\ 0 & 0 & 0 & 0 & 0 & 0 \\ 0 & 0 & 0 & 0 & 0 & 0 \\ 0 & 0 & 0 & 0 & 0 & 0 \end{pmatrix} + \begin{pmatrix} 0 & 0 & 0 & 0 & 0 & 0 \\ 0 & 0 & 1 & 0 & 0 & 0 \\ 0 & 1 & 0 & 0 & 0 & 0 \\ 0 & 0 & 0 & 0 & 0 & 0 \\ 0 & 0 & 0 & 0 & 0 & 0 \\ 0 & 0 & 0 & 0 & 0 & 0 \end{pmatrix} + \begin{pmatrix} 0 & 0 & 0 & 0 & 0 & 0 \\ 0 & 0 & 0 & 1 & 0 & 0 \\ 0 & 0 & 0 & 0 & 0 & 0 \\ 0 & 1 & 0 & 0 & 0 & 1 \\ 0 & 0 & 0 & 0 & 0 & 0 \\ 0 & 0 & 0 & 1 & 0 & 0 \end{pmatrix}$$

$$+ \begin{pmatrix} 0 & 0 & 0 & 0 & 0 & 0 \\ 0 & 0 & 0 & 0 & 0 & 0 \\ 0 & 0 & 0 & 0 & 0 & 0 \\ 0 & 0 & 0 & 0 & 1 & 0 \\ 0 & 0 & 0 & 1 & 0 & 0 \\ 0 & 0 & 0 & 0 & 0 & 0 \end{pmatrix} + \begin{pmatrix} 0 & 0 & 0 & 0 & 0 & 0 \\ 0 & 0 & 0 & 0 & 0 & 0 \\ 0 & 0 & 0 & 0 & 0 & 0 \\ 0 & 0 & 0 & 0 & 0 & 0 \\ 0 & 0 & 0 & 0 & 0 & 1 \\ 0 & 0 & 0 & 0 & 1 & 0 \end{pmatrix}$$

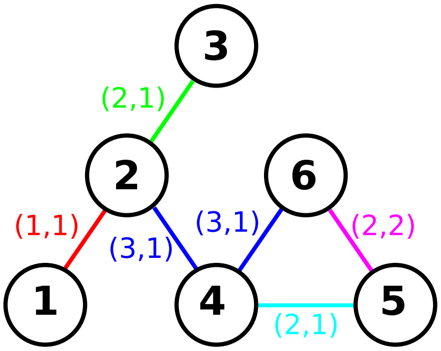


FIG. 3. Example of a matrix after step 1 of the edge coloring algorithm, which uses only nearest neighbor information. The edges are colored as outlined by the algorithm, and the matrix is decomposed into separate parts for each color. After this step, most sub-matrices are one-sparse, however as seen one matrix still contains a two-sparse structure.

manner. For each $x_l^{(0)}$ and $x_{l+1}^{(0)}$, determine the first bit position (bits are numbered from left to right) where the two numbers differ. Record the value of this bit in $x_l^{(0)}$, and set $x_l^{(1)}$ to be this bit value at the far left bit position, followed by the binary representation of the location of this bit. The bits are numbered from left to right, and the first bit is numbered $00\cdots 0$. If $x_l^{(0)}$ is at the end of the sequence, simply set $x_l^{(1)}$ to be the first bit value of $x_l^{(0)}$ followed by the binary representation of 0. The number of bits needed to represent $x_l^{(1)}$ is $\log_2(2n)$ where $n$ is the number of bits needed to represent all $x_l^{(0)}$ vertices. After at most $k = \log^* N$ iterations, each $x_l^{(k)}$ in the sequence will be different from its neighbor and there will be at most 6 unique values. Once the $x_l^{(k)}$ values cease changing, the algorithm terminates and we swap the first and last bits to ensure that the six unique values are $x_l^{(k)} \leq 5$.

Table I shows the deterministic coin tossing algorithm for the $6 \times 6$ example that we have been working with. We use two examples: the first being a simple single edge coloring for $(1, 2)$, and the second being the slightly more involved coloring for the two connected edges $(2, 4)$ and $(4, 6)$. At iteration 0, each edge is simply labeled with the vertex of lower number. Each column in the table is an iteration of the coin-tossing algorithm.

The final edge-colored output of the $6 \times 6$ example is shown in Fig. 4. One sees that in fact each sub-Hamiltonian

| Vertex Chain | Iter 0 | Iter 1 | Iter 2 | Iter 3 | Iter 4 | Swap |
|---|---|---|---|---|---|---|
| 1 | 001 | 001 | 110 | 100 | 100 | 001 |
| 2 | 010 | 000 | 000 | 000 | 000 | 000 |
| 2 | 010 | 000 | 010 | 101 | 100 | 001 |
| 4 | 100 | 001 | 000 | 000 | 000 | 000 |
| 6 | 110 | 100 | 100 | 100 | 100 | 001 |

TABLE I. Deterministic coin tossing example for edge $(1,2)$ and edges $(2,4) \to (4,6)$. By applying the algorithm outlined in this section one can arrive at a one-sparse edge coloring. The vertex chain column corresponds to the chain indicated in Eq. (50), and each iteration is an update of the chain coloring. The edge is finally colored with the label given by the vertex of lower number (i.e. edge $(1,2)$ is colored 001, edge $(2,4)$ is colored 001, and edge $(4,6)$ is colored 000).

is indeed one-sparse.

$$A = \begin{pmatrix} 0&1&0&0&0&0\\ 1&0&0&0&0&0\\ 0&0&0&0&0&0\\ 0&0&0&0&0&0\\ 0&0&0&0&0&0\\ 0&0&0&0&0&0 \end{pmatrix} + \begin{pmatrix} 0&0&0&0&0&0\\ 0&0&1&0&0&0\\ 0&1&0&0&0&0\\ 0&0&0&0&0&0\\ 0&0&0&0&0&0\\ 0&0&0&0&0&0 \end{pmatrix} + \begin{pmatrix} 0&0&0&0&0&0\\ 0&0&0&1&0&0\\ 0&0&0&0&0&0\\ 0&1&0&0&0&0\\ 0&0&0&0&0&0\\ 0&0&0&0&0&0 \end{pmatrix}$$
$$+ \begin{pmatrix} 0&0&0&0&0&0\\ 0&0&0&0&0&0\\ 0&0&0&0&0&0\\ 0&0&0&0&1&0\\ 0&0&0&1&0&0\\ 0&0&0&0&0&0 \end{pmatrix} + \begin{pmatrix} 0&0&0&0&0&0\\ 0&0&0&0&0&0\\ 0&0&0&0&0&0\\ 0&0&0&0&0&0\\ 0&0&0&0&0&1\\ 0&0&0&0&1&0 \end{pmatrix} + \begin{pmatrix} 0&0&0&0&0&0\\ 0&0&0&0&0&0\\ 0&0&0&0&0&0\\ 0&0&0&0&0&1\\ 0&0&0&0&0&0\\ 0&0&0&1&0&0 \end{pmatrix}$$

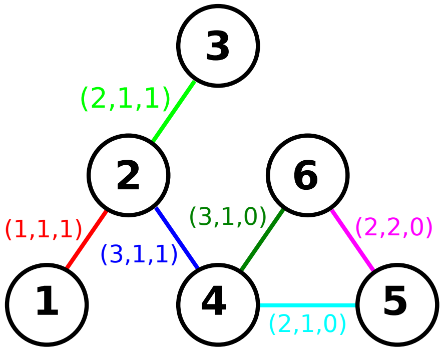


FIG. 4. Example of a matrix decomposition after deterministic coin-tossing portion of edge-coloring algorithm. The edges are colored as outlined by the algorithm, and the matrix is decomposed into separate parts for each color. After this step, all sub-matrices are correctly one-sparse, and thus can be efficiently simulated.

### *3. Banded Matrix Hamiltonian Decomposition*

As an aside, in our toy scattering model that we show later, the decomposition problem is much simpler than the graph coloring method just presented. For arbitrarily sized finite elements, the location of the matrix entries are unknown. However, for uniform finite element grids of square elements the matrix is banded, and the number and location of the bands is given by the geometry of the scattering problem. Therefore we know where the non-zero matrix elements are restricted to lie. This enables for a vast simplification when decomposing the matrix $A$.

To decompose the matrix, we simply choose to break up the matrix by band. Thus we take

$$A = \sum_{c=1}^{N_b} A_c, \tag{51}$$

where $A_c$ is the $c^{th}$ non-zero band of matrix $A$, and $N_b$ is the number of bands in matrix $A$. For square finite element grids, which we use in this example, $N_b = 9$. Because the location of the bands are known, this method to decompose the matrix $A$ takes $O(1)$ time. We note that the banded nature of the matrix does not necessarily carry over when using the preconditioned method. One can impose sparsity constraints on the precondition matrix $MA$ to ensure this, but one typically allows the sparsity structure to vary, allowing for more efficient preconditioners.

### *4. Hamiltonian Circuit*

We will now describe a quantum circuit which will apply a one-sparse Hamiltonian to an arbitrary state. The procedure is a generalization of the quantum random walk algorithm [13–15]. We define two operators, one to calculate the magnitude and one to calculate the phase, of a particular 1-sparse matrix $A_c$

$$U_m^{(c)}|a\rangle_2|b\rangle_3|y\rangle_4|z\rangle_5 = |a\rangle_2|b\oplus v_c(a)\rangle_3|y\oplus x_c(a)\rangle_4|z\rangle_5 \tag{52}$$
$$U_p^{(c)}|a\rangle_2|b\rangle_3|y\rangle_4|z\rangle_5 = |a\rangle_2|b\oplus v_c(a)\rangle_3|y\rangle_4|z\oplus \phi_c(a)\rangle_5$$

where $a$ is the row index, $c$ is a color index ranging from 1 to $6d^2$ representing the desired sub-matrix, $v_c(a)$ is the vertex connected to $a$ in sub-matrix $c$, $x_c(a) = |\langle a|A_c|v_c(a)\rangle|$ is the magnitude of the matrix element associated with this transition, and $\phi_c(a) = \text{phase}(\langle a|A_c|v_c(a)\rangle)$ is the complex phase of the matrix element. This unitary can be implemented with $O(\log^* N)$ calls to the oracle as shown in the previous section. If no state is connected to vertex $a$ in sub-matrix $c$, then $v_c(a) = x_c(a) = \phi_c(a) = 0$. It is straightforward to verify that $U_m^{(c)\dagger} = U_m^{(c)}$ and $U_p^{(c)\dagger} = U_p^{(c)}$.

We define the action of a second operator as

$$H_{rw}|a\rangle_2|b\rangle_3|y\rangle_4|\phi\rangle_5 = y|b\rangle_2|a\rangle_3|y\rangle_4|\phi\rangle_5. \tag{53}$$

We refer to this operator as $H_{rw}$ because of its similarity with the quantum walk Hamiltonian [14]. This operator swaps registers 2 and 3 and is diagonal in the third register. This operator can be written as

$$H_{rw} = \left(\bigotimes_{l=1}^{n} S^{l,n+l}\right)_{2,3} \otimes \sum_y y|y\rangle_4\langle y|_4, \tag{54}$$

where $S^{l,n+l}$ is applied to registers 2 and 3 and simply swaps bits $l$ and $n+l$ or the $l^{\text{th}}$ bit of register 2 and the $l^{\text{th}}$ bit of register 3 since both are $n$ bit registers and the second operator is applied to register 4. In the $l$, $n+l$ two-qubit sub-space, the swap operator is

$$S^{l,n+l} = \begin{pmatrix} 1 & 0 & 0 & 0 \\ 0 & 0 & 1 & 0 \\ 0 & 1 & 0 & 0 \\ 0 & 0 & 0 & 1 \end{pmatrix}, \tag{55}$$

and it is diagonalized via

$$W = \begin{pmatrix} 1 & 0 & 0 & 0 \\ 0 & \frac{1}{\sqrt{2}} & \frac{1}{\sqrt{2}} & 0 \\ 0 & \frac{1}{\sqrt{2}} & -\frac{1}{\sqrt{2}} & 0 \\ 0 & 0 & 0 & 1 \end{pmatrix}, \tag{56}$$

with eigenvalues $(1, 1, -1, 1)$. The operator $W$ can be implemented with the circuit in Fig. 5.

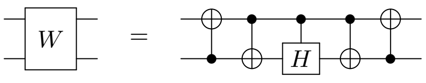


FIG. 5. Quantum circuit to implement $W$.

Next we define a controlled phase gate. The action of a controlled phase gate is

$$P|\phi\rangle_5|0\rangle_6 = e^{i\phi/2}|\phi\rangle_5|0\rangle_6, \tag{57}$$

which takes the value stored in register 5 and applies it as a phase to the state. Register 5 contains the value of the phase stored as an integer multiple of some minimal phase shift, denoted $\phi_0$. Register 6 is a single ancilla qubit. The circuit representation of Eq. (57) is

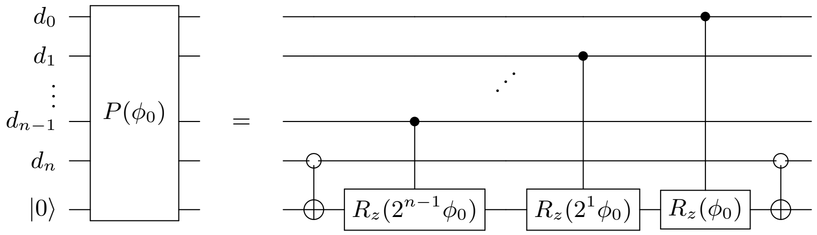


FIG. 6. Circuit to implement Eq. (57). The gate $R_z(\theta)$ is defined on p. 174 of Ref. [16], and $\phi_0$ is the minimum phase shift for the particular circuit.

Using these operators the $A$ matrix can be written as

$$A = \sum_{c=1}^{N_b} A_c = \sum_{c=1}^{N_b} U_p^{(c)} P^\dagger U_p^{(c)} U_m^{(c)} H_{rw} U_m^{(c)} U_p^{(c)} P U_p^{(c)} \tag{58}$$

which when restricted to acting on the subspace of initial states $|a, 0, 0, 0\rangle$ gives

$$\begin{aligned}
A|a\rangle_2|0\rangle_3|0\rangle_4|0\rangle_5 &= \sum_{c=1}^{N_b} U_p^{(c)} P^\dagger U_p^{(c)} U_m^{(c)} H_{rw} U_m^{(c)} U_p^{(c)} P U_p^{(c)} |a\rangle_2|0\rangle_3|0\rangle_4|0\rangle_5 \\
&= \sum_{c=1}^{N_b} U_p^{(c)} P^\dagger U_p^{(c)} U_m^{(c)} H_{rw} U_m^{(c)} U_p^{(c)} P |a\rangle_2|v_c(a)\rangle_3|0\rangle_4|\phi_c(a)\rangle_5 \\
&= \sum_{c=1}^{N_b} e^{i\phi_c(a)/2} U_p^{(c)} P^\dagger U_p^{(c)} U_m^{(c)} H_{rw} U_m^{(c)} |a\rangle_2|0\rangle_3|0\rangle_4|0\rangle_5 \\
&= \sum_{c=1}^{N_b} e^{i\phi_c(a)/2} U_p^{(c)} P^\dagger U_p^{(c)} U_m^{(c)} H_{rw} |a\rangle_2|v_c(a)\rangle_3|x_c(a)\rangle_4|0\rangle_5 \\
&= \sum_{c=1}^{N_b} x_c(a) e^{i\phi_c(a)/2} U_p^{(c)} P^\dagger U_p^{(c)} U_m^{(c)} |v_c(a)\rangle_2|a\rangle_3|x_c(a)\rangle_4|0\rangle_5 \\
&= \sum_{c=1}^{N_b} x_c(a) e^{i\phi_c(a)/2} U_p^{(c)} P^\dagger U_p^{(c)} |v_c(a)\rangle_2|0\rangle_3|0\rangle_4|0\rangle_5 \\
&= \sum_{c=1}^{N_b} x_c(a) e^{i\phi_c(a)/2} U_p^{(c)} P^\dagger |v_c(a)\rangle_2|a\rangle_3|0\rangle_4|-\phi_c(a)\rangle_5 \\
&= \sum_{c=1}^{N_b} x_c(a) e^{i\phi_c(a)} U_p^{(c)} |v_c(a)\rangle_2|a\rangle_3|0\rangle_4|-\phi_c(a)\rangle_5 \\
&= \sum_{c=1}^{N_b} x_c(a) e^{i\phi_c(a)} |v_c(a)\rangle_2|0\rangle_3|0\rangle_4|0\rangle_5
\end{aligned} \tag{59}$$

,

where we have used the fact that $A$ is Hermitian and thus $v_c(v_c(a)) = a$, $x_c(v_c(a)) = x_c(a)$, and $\phi_c(v_c(a)) = -\phi_c(a)$. From Eq. (59) one can clearly see that the matrix as written in Eq. (58) is a valid decomposition of the $A$ matrix into elementary operations.

Next, we demonstrate how to implement $e^{-iA_ct}$ as a quantum circuit, which is required for Hamiltonian simulation. Since $U_m^{(c)}U_m^{(c)} = U_p^{(c)}U_m^{(c)} = 1$ and $P^\dagger P = 1$, we can write $e^{-iA_ct} = U_p^{(c)}P^\dagger U_p^{(c)}U_m^{(c)}e^{-iH_{rw}t}U_m^{(c)}U_p^{(c)}PU_p^{(c)}$, thus we only need to demonstrate a circuit for simulating $e^{-iH_{rw}t}$. When the Hamiltonian weights are restricted to $x_c(a) = 0$ or $x_c(a) = 1$ we have a quantum walk, so our circuit will be similar to the one given in [14]. The generalized quantum walk circuit implementation, including non-binary weights, is shown in Fig. 7. This circuit implements

$$\begin{aligned} M|a, v_c(a), x_c(a), \phi_c(a)\rangle &= e^{-iH_{rw}t}|a, v_c(a), x_c(a), \phi_c(a)\rangle \\ &= \cos(x_c(a)t)|a, v_c(a), x_c(a), \phi_c(a)\rangle - i\sin(x_c(a)t)|v_c(a), a, x_c(a), \phi_c(a)\rangle. \end{aligned} \tag{60}$$

Combining this circuit with the unitary operations which compute the various weights allows one to simulate $e^{-iA_ct}$. The circuit to simulate

$$e^{-iA_ct}|a, 0, 0, 0\rangle = \cos(x_c(a)t)|a, 0, 0, 0\rangle - i\sin(x_c(a)t)e^{i\phi_c(a)}|v_c(a), 0, 0, 0\rangle \tag{61}$$

is given in Fig. 8.

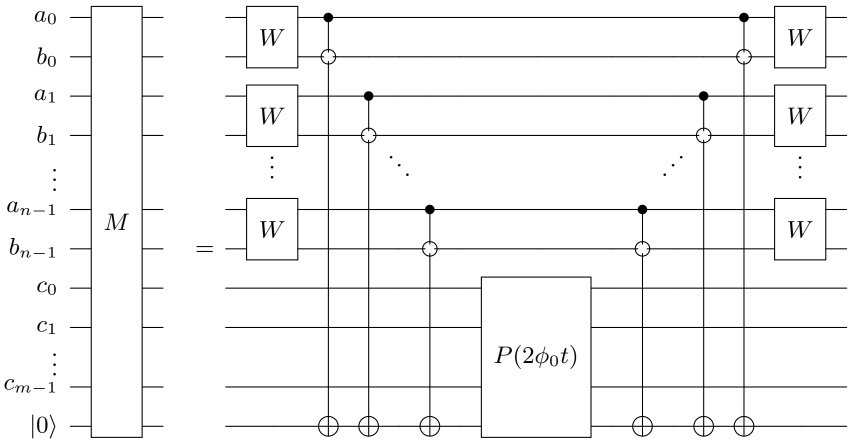


FIG. 7. Quantum circuit to implement Eq. (60). The term $\phi_0$ is the minimum phase shift for the circuit.

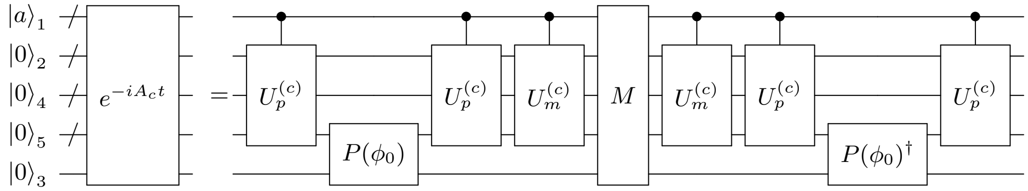


FIG. 8. Quantum circuit to implement Eq. (61). The term $\phi_0$ is the minimum phase shift for the circuit. The $M$ circuit is given in Fig. 7 and the $P$ circuit is given in Fig. 6.

## IV. ORACLES FOR ELECTROMAGNETIC SCATTERING APPLICATION

The finite element method can be used to solve Maxwell's equations by converting them into a sparse linear system [17]. In this section we will demonstrate how to design the quantum oracles required by the QLSA for an electromagnetic scattering problem. Three oracles will be presented. The first two are used to calculate the matrix elements of the unpreconditioned matrix $A$ and the initial state $|b\rangle$. These are presented in section IV A. The third, which is used for creation of the state $|R\rangle$, is explained in IV B.

Again, the scattering problem we demonstrate is meant as an example. We choose a simple finite element geometry, and we choose first order absorbing boundary conditions together with a metallic scatterer. None of these choices are required by the quantum algorithm, and the problem can be generalized as desired. They are chosen simply for illustrative purposes.

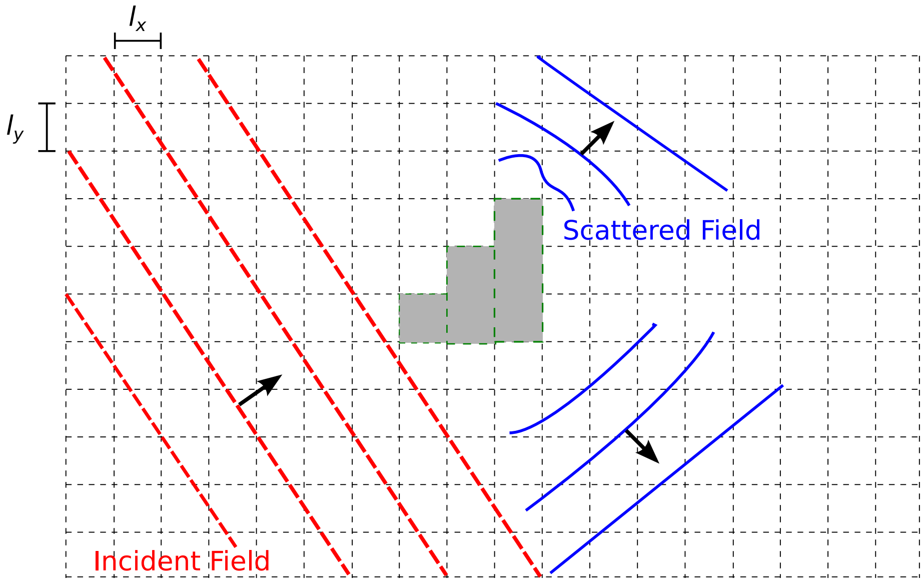


FIG. 9. Two-dimensional finite element mesh with square finite elements. The scattering region is shown in grey, and can be any arbitrary design. The incident field interacts with the metallic scatterer and scatters off into all directions.

### A. $A$ Matrix and $|b\rangle$ Vector Oracles

The basic principle of the finite element method (FEM) is to break up the computational domain into small volume elements. Typically, these are tetrahedral or brick shaped elements. One of the strengths of the FEM is that the technique allows for non-uniform meshes, meaning meshes can be more dense in areas where high accuracy is needed and less dense when lower accuracy is sufficient. However one of the key constraints with the QLSA is that the matrix elements must be efficiently computable. This restricts one to semi-regular or functionally defined meshes.

As a simple toy–problem example, we will model the scattering of a plane wave off an arbitrary 2D metallic scattering region with a uniform rectangular mesh, as shown in Fig. 9. Following standard FEM techniques[17], we write the free-space Maxwell's equation as a functional

$$F(\boldsymbol{E}) = \int_V \left[(\nabla \times \boldsymbol{E}) \cdot (\nabla \times \boldsymbol{E}) - k^2 \boldsymbol{E} \cdot \boldsymbol{E}\right] dV + ik \int_S \boldsymbol{E}_t \cdot \boldsymbol{E}_t dS, \tag{62}$$

where

$$\mathbf{E}(x, y) = E_0 \hat{\boldsymbol{p}} e^{-i\mathbf{k}\cdot\mathbf{r}(x,y)} \tag{63}$$

is the vector electromagnetic field propagating in direction $\hat{k} = \mathbf{k}/k = \cos\theta\hat{\boldsymbol{x}} + \sin\theta\hat{\boldsymbol{y}}$, at position $\mathbf{r}(x, y) = x\hat{\boldsymbol{x}} + y\hat{\boldsymbol{y}}$, with magnitude $E_0$, wavenumber $k$, and polarization $\hat{p} = \hat{\boldsymbol{r}} \times \hat{\boldsymbol{z}}$. The label $\boldsymbol{E}_t$ indicates the component tangential to the surface $S$, $V$ is the volume of the computational region, and $S$ is the outer surface of the computational region. By taking $\delta F = 0$, the volume term gives Maxwell's equation for the electric field, while the surface integral is an artificial absorbing term used to prevent reflections off the artificial computational boundary. On the inner metallic scattering surface the boundary condition

$$\hat{n} \times \boldsymbol{E} = -\hat{n} \times \boldsymbol{E}^i \tag{64}$$

where $\boldsymbol{E}^i$ is the incident field, and $\hat{n}$ is the unit vector normal to the surface is applied.

Within an element labelled $e$ the electric field can be expanded in terms of edge basis vectors [18],

$$\boldsymbol{E}^e = \sum_{i=1}^{4} \boldsymbol{N}_i^e e_i^e \tag{65}$$

where $e_i^e$ is the magnitude of the electric field along edge $i$ and

$$\boldsymbol{N}_1^e = \frac{1}{l_y}\left(y_c^e + \frac{l_y}{2} - y\right)\hat{x} \qquad \boldsymbol{N}_2^e = \frac{1}{l_y}\left(y - y_c^e + \frac{l_y}{2}\right)\hat{x} \tag{66}$$
$$\boldsymbol{N}_3^e = \frac{1}{l_x}\left(x_c^e + \frac{l_x}{2} - x\right)\hat{y} \qquad \boldsymbol{N}_3^e = \frac{1}{l_x}\left(x - x_c^e + \frac{l_x}{2}\right)\hat{x},$$

where $(x_c^e, y_c^e)$ is the coordinates of the center of the element, and $l_{x,y}$ are the lengths of the $x, y$ edges. It is straightforward to show that $\nabla \cdot \boldsymbol{N}_i^e = 0$ which implies $\nabla \cdot \boldsymbol{E}^e = 0$ constant curl

$$\nabla \times \boldsymbol{N}_1^e = \frac{1}{l_y}\hat{z} \qquad \nabla \times \boldsymbol{N}_2^e = -\frac{1}{l_y}\hat{z} \tag{67}$$
$$\nabla \times \boldsymbol{N}_3^e = -\frac{1}{l_x}\hat{z} \qquad \nabla \times \boldsymbol{N}_3^e = \frac{1}{l_x}\hat{z}.$$

Thus these are valid basis functions to use for the electric field. Using these relationships and the expansion of the field given in Eq. (65), Eq. (62) can be written as

$$F(\boldsymbol{E}) = \sum_{e=1}^{n_e}\sum_{i=1}^{4}\sum_{i'=1}^{4}\int_{V_e}\left[(\nabla \times \boldsymbol{N}_i^e e_i^e)\cdot(\nabla \times \boldsymbol{N}_{i'}^e e_{i'}^e) - k^2 \boldsymbol{N}_i^e e_i^e \cdot \boldsymbol{N}_{i'}^e e_{i'}^e\right] dV \tag{68}$$
$$+ ik \sum_{e=1}^{n_e}\sum_{i=1}^{4}\sum_{i'=1}^{4}\int_{S_e}(\boldsymbol{N}_i^e e_i^e)_t \cdot (\boldsymbol{N}_{i'}^e e_{i'}^e)_t dS,$$

where $n_e$ is the number of finite elements, $V_e$ is the volumetric region for element $e$, and $S_e$ is the surface region of element $e$. Note that there is only a single sum over the finite elements $e$. This is due to the local nature of the finite element basis vectors.

Next, the minimum is computed by taking the derivative with respect to $e_k$ and set equal to 0. This gives

$$\frac{\partial F}{\partial e_k} = \sum_j \int_V \left[(\nabla \times \boldsymbol{N}_k)\cdot(\nabla \times \boldsymbol{N}_j) - k^2 \boldsymbol{N}_k \cdot \boldsymbol{N}_j\right] e_j dV + ik \sum_j \int_S (\boldsymbol{N}_k)_t \cdot (\boldsymbol{N}_j)_t e_j dS = 0, \tag{69}$$

which can be written more simply as $\sum_j F_{kj} e_j = 0$ with

$$F_{kj} = \int_V \left[(\nabla \times \boldsymbol{N}_k)\cdot(\nabla \times \boldsymbol{N}_j) - k^2 \boldsymbol{N}_k \cdot \boldsymbol{N}_j\right] dV + ik \int_S (\boldsymbol{N}_k)_t \cdot (\boldsymbol{N}_j)_t dS. \tag{70}$$

Because of the local nature of the finite element expansion, the volume and surface integrals extend only over the region encompassed by the finite element. As a result $F_{kj}$ is a highly sparse matrix. For rectangular finite elements the maximum number of non-zero elements in a given row is 7. In addition, for regular grids, the matrix is banded with a total of 9 bands. We will compute the volume and surface integral portions of $F_{ij}$ separately and denote them by $B_{ij}$ and $C_{ij}$ respectively.

First the volume integrals are calculated using the edge labeling scheme shown in Fig. 10(a). These are

$$B_{11}^e = B_{22}^e = \frac{l_x}{l_y} - k^2 \frac{l_x l_y}{3} \qquad B_{33}^e = B_{44}^e = \frac{l_y}{l_x} - k^2 \frac{l_x l_y}{3} \tag{71}$$
$$B_{12}^e = -\frac{l_x}{l_y} + k^2 \frac{l_x l_y}{12} \qquad B_{34}^e = -\frac{l_y}{l_x} + k^2 \frac{l_x l_y}{12}$$
$$B_{13}^e = B_{24}^e = -1 \qquad B_{14}^e = B_{23}^e = 1.$$

The corresponding surface integrals are

$$C_{11}^e = C_{22}^e = ikl_x \quad C_{33}^e = C_{44}^e = ikl_y \quad C_{i\neq j}^e = 0. \tag{72}$$

The known field values on the internal scattering surface are given in Eq. (64) and should be moved to the right hand side of Eq. (69). We will denote the indices from 1 to $N$ as the global edge indices, where the numbering scheme is shown in Fig. 10(b). Construct the $N \times N$ diagonal matrix $D$ whose elements are 1 for free edges, and 0 for edges on or inside the scattering body. This allows us to rewrite Eq. (69) as

$$Ae = b, \tag{73}$$

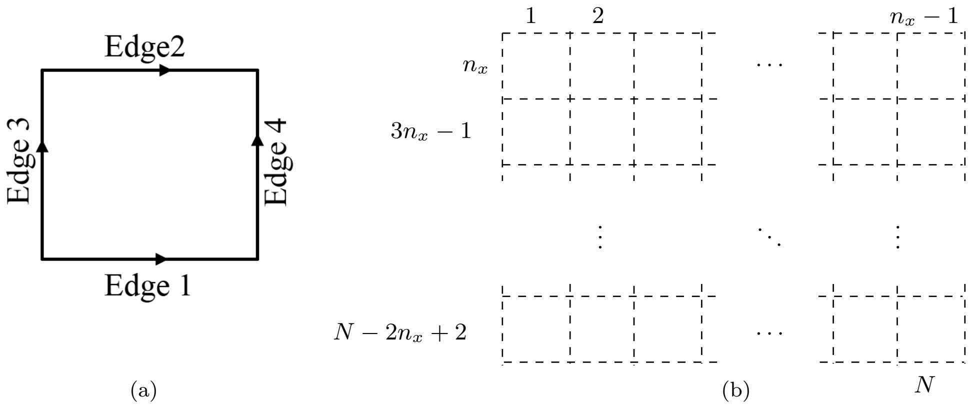


FIG. 10. Finite Element numbering scheme. (a) The local numbering scheme we use to define the integrals in Eqs. (71) and (72). (b) The global numbering scheme that we use to populate our scattering matrix. The total number of edges are $N = n_x(n_y - 1) + n_y(n_x - 1)$.

where

$$A = DFD + \mathbb{I} - D \qquad \text{and} \qquad b = [DF(D - \mathbb{I}) + (D - \mathbb{I})]e, \tag{74}$$

where $\mathbb{I}$ is the identity matrix. In writing $A$ and $b$ in this form, one can verify that all edge values known from boundary conditions are on the right hand side, and all unknown edge values to be solved for reside on the left hand side. In addition all matrix elements are efficiently computable by using Eqs. (71) and (72) together with (74).

We can now define the quantum oracle, which is required to compute the unpreconditioned $A$ matrix. It is

$$f(y,i) = \begin{cases} [B^e_{m(y)m(x(y,i))} + C^e_{m(y)m(x(y,i))}, N + x(y,i)] & \text{if } y < N \\ [B^e_{m(x(y-N,i))m(y-N)} - C^e_{m(x(y-N,i))m(y-N)}, x(y-N,i)] & \text{if } y \geq N \end{cases} \tag{75}$$

where $m(y)$ is a mapping which converts a global edge index, $1 \leq y < N$, to its local edge index which is numbered between 1 and 4, as shown in Fig. 9, and $x(y,i)$ is the global edge index corresponding to the edge in the $i^{th}$ band connected to $y$. The $B_{ij}$ and $C_{ij}$ terms are defined in Eqs. (71) and (72). The reason for the two terms in the oracle is to ensure unitarity of the Hamiltonian simulation operator. As defined, the oracle creates the matrix

$$\mathcal{A} = \begin{pmatrix} 0 & A \\ A^\dagger & 0 \end{pmatrix}, \tag{76}$$

which is always Hermitian. More information in this reduction is available in [1].

The $|b\rangle$ vector oracle, required to compute the unpreconditioned $b_j$ elements of $|b\rangle = \sum_j b_j |j\rangle$ can also now be defined. It is

$$b_j = \begin{cases} \sum_{k=1}^{N_c} f_k B^e_{m(j)m'(j,k)} \mathbf{E}(x_k, y_k) \cdot \hat{\boldsymbol{l}}_k & \text{if } j < N \\ 0 & \text{otherwise,} \end{cases} \tag{77}$$

where $N_c < 7$ is maximum number of metallic edges connected to edge $j$, $f_k$ is a flag with value 1 or 0 indicating whether edge $k$ is or is not a metallic edge with known field value, $m'(j,k)$ is a mapping from global index $j$ and connectivity index $k$ to its local element index, $\mathbf{E}$ is the electric field defined in Eq. (63), $(x_k, y_k)$ are the physical coordinates of edge $k$, and $\hat{\boldsymbol{l}}_k$ is the unit vector in the direction of edge $k$.

### B. $|R\rangle$ Vector Oracle

Given the fields $\boldsymbol{E}(\mathbf{r})$ from (65) and $\boldsymbol{H}(\mathbf{r}) = -(i\omega\mu_0)^{-1}\nabla \times \boldsymbol{E}(\mathbf{r})$ for $\mathbf{r} \in S$, the radiated electric field in the far-field is given by

$$\boldsymbol{E}(\mathbf{s}) \approx \frac{e^{-iks}}{4\pi s} \int_S \{ i\omega\mu_0 \widehat{\mathbf{s}} \times [\widehat{\mathbf{s}} \times \boldsymbol{J}(\mathbf{r})] + ik\widehat{\mathbf{s}} \times \boldsymbol{M}(\mathbf{r}) \} \, e^{ik\widehat{\mathbf{s}}\cdot\mathbf{r}} \, dS, \tag{78}$$

where $\boldsymbol{J}(\mathbf{r}) \equiv \widehat{\mathbf{n}}(\mathbf{r}) \times \boldsymbol{H}(\mathbf{r})$ and $\boldsymbol{M}(\mathbf{r}) \equiv \boldsymbol{E}(\mathbf{r}) \times \widehat{\mathbf{n}}(\mathbf{r})$, with $\widehat{\mathbf{n}}(\mathbf{r})$ the unit normal of the surface $S$ at $\mathbf{r}$. Subsituting (65) into (78) gives

$$\mathbf{E}(\mathbf{s}) \cdot \widehat{\mathbf{p}} \approx \frac{e^{-iks}}{4\pi s} \sum_k R_k(\widehat{\mathbf{s}}) e_k, \tag{79}$$

where $\widehat{\mathbf{p}}$ is the radar polarization (with $\widehat{\mathbf{p}} \cdot \widehat{\mathbf{s}} = 0$) and

$$R_k(\widehat{\mathbf{s}}, \widehat{\mathbf{p}}) \equiv \widehat{\mathbf{p}} \cdot \int_S \widehat{\mathbf{s}} \times \{\widehat{\mathbf{s}} \times [(\nabla \times \boldsymbol{N}_k) \times \widehat{\mathbf{n}}] + ik\boldsymbol{N}_k \times \widehat{\mathbf{n}}\} \, e^{ik\widehat{\mathbf{s}}\cdot\mathbf{r}} \, dS, \tag{80}$$

where the index $k$ here is the global edge index. The radar cross-section (RCS) in the direction $\widehat{\mathbf{s}}$ is given by

$$\mathrm{RCS} = \lim_{s\to\infty} 4\pi s^2 |\mathbf{E}(\mathbf{s}) \cdot \widehat{\mathbf{p}}|^2 = \frac{1}{4\pi} \left| \sum_k R_k e_k \right|^2 \equiv \frac{1}{4\pi} |\langle R|x\rangle|^2. \tag{81}$$

Thus, the radar cross section is simply the dot product of vector $R_k$ with the vector $e_k$. Thus one sees how the QLSA outlined in Section II can be used to calculate the radar cross section of a metallic scattering region.

The vector $R_k$ can be computed by once again using the definition of the vector $\boldsymbol{N}_k$. There are four separate surface terms (for each of the four edges), giving the following terms needed to compute $R_k$

$$\begin{aligned}
R_1^e &= \frac{I_1^e}{l_y} \left[\cos\phi(\sin\phi + ikl_y)\widehat{\mathbf{y}} - \sin\phi(\sin\phi + ikl_y)\widehat{\mathbf{x}}\right] \cdot \widehat{\mathbf{p}} \\
R_2^e &= \frac{I_2^e}{l_y} \left[\cos\phi(\sin\phi - ikl_y)\widehat{\mathbf{y}} - \sin\phi(\sin\phi - ikl_y)\widehat{\mathbf{x}}\right] \cdot \widehat{\mathbf{p}} \\
R_3^e &= \frac{I_2^e}{l_x} \left[-\cos\phi(\cos\phi + ikl_x)\widehat{\mathbf{y}} + \sin\phi(\cos\phi + ikl_x)\widehat{\mathbf{x}}\right] \cdot \widehat{\mathbf{p}} \\
R_4^e &= \frac{I_2^e}{l_x} \left[-\cos\phi(\cos\phi - ikl_x)\widehat{\mathbf{y}} + \sin\phi(\cos\phi - ikl_x)\widehat{\mathbf{x}}\right] \cdot \widehat{\mathbf{p}},
\end{aligned} \tag{82}$$

where we have taken $\widehat{\mathbf{s}} = \cos\phi\widehat{\mathbf{x}} + \sin\phi\widehat{\mathbf{y}}$, and the terms $I_i$ are given by

$$\begin{aligned}
I_1^e &= l_x e^{ik(y_c^e - l_y/2)\sin\phi} e^{ikx_c^e \cos\phi} \operatorname{sinc} \frac{kl_x \cos\phi}{2} \\
I_2^e &= l_x e^{ik(y_c^e + l_y/2)\sin\phi} e^{ikx_c^e \cos\phi} \operatorname{sinc} \frac{kl_x \cos\phi}{2} \\
I_3^e &= l_y e^{ik(x_c^e - l_x/2)\cos\phi} e^{iky_c^e \sin\phi} \operatorname{sinc} \frac{kl_y \sin\phi}{2} \\
I_4^e &= l_y e^{ik(x_c^e + l_x/2)\cos\phi} e^{iky_c^e \sin\phi} \operatorname{sinc} \frac{kl_y \sin\phi}{2},
\end{aligned} \tag{83}$$

where $\mathrm{sinc\,x} = \mathrm{sin\,x/x}$. Thus the oracle function is simply

$$r_j = \begin{cases} R^e_{m(j-N)} & \text{if } j \text{ is an outside edge and } j \geq N \\ 0 & \text{otherwise,} \end{cases} \tag{84}$$

where $m(j)$ is the same mapping function defined for the $A$ and $|b\rangle$ oracles.

## ACKNOWLEDGMENTS

This project was supported by the Intelligence Advanced Research Projects Activity via Department of Interior National Business Center contract numbers N00024-03-D-6606 and 2012-12050800010, with additional support provided by a Stuart S. Janney Fellowship from the Applied Physics Laboratory. The U.S. Government is authorized to reproduce and distribute reprints for Governmental purposes notwithstanding any copyright annotation thereon. The

views and conclusions contained herein are those of the authors and should not be interpreted as necessarily representing the official policies or endorsements, either expressed or implied, of IARPA, DoI/NBC, or the U.S. Government. Many thanks to Joan Hoffmann and Nathan Wiebe for helpful comments and discussions.

[1] A. W. Harrow, A. Hassidim, and S. Lloyd, Phys. Rev. Lett., **103**, 150502 (2009).
[2] G. Brassard, P. Hoyer, M. Mosca, and A. Tapp, arXiv.org:quant-ph/0005055 (2000).
[3] D. Berry, G. Ahokas, R. Cleve, and B. Sanders, Communications in Mathematical Physics, **270**, 359 (2007).
[4] L. Grover and T. Rudolph, arXiv:quant-ph/0208112v1 (2002).
[5] D. Aharonov and A. Ta-Shma, in *Proceedings of the thirty-fifth annual ACM symposium on Theory of computing*, STOC '03 (ACM, New York, NY, USA, 2003) pp. 20–29.
[6] N. J. Ward, I. Kassal, and A. Aspuru-Guzik, The Journal of Chemical Physics, **130**, 194105 (2009).
[7] A. N. Soklakov and R. Schack, Phys. Rev. A, **73**, 012307 (2006).
[8] P. Kaye and M. Mosca, arXiv:quant-ph/0407102v1 (2004).
[9] M. Suzuki, Physics Letters A, **146**, 319 (1990).
[10] H. F. Trotter, Proceedings of the American Mathematical Society, 545 (1959).
[11] R. Cole and U. Vishkin, Information and Control, **70**, 32 (1986).
[12] A. V. Goldberg, S. A. Plotkin, and G. E. Shannon, SIAM Journal on Discrete Mathematics, **1**, 434 (1988).
[13] D. Aharonov and A. Ta-Shma, in *Proceedings of the thirty-fifth annual ACM symposium on Theory of computing* (ACM, 2003) pp. 20–29.
[14] A. M. Childs, R. Cleve, E. Deotto, E. Farhi, S. Gutmann, and D. A. Spielman, in *Proceedings of the thirty-fifth annual ACM symposium on Theory of computing*, STOC '03 (ACM, New York, NY, USA, 2003) pp. 59–68, ISBN 1-58113-674-9.
[15] N. Wiebe, D. W. Berry, P. Hoyer, and B. C. Sanders, Journal of Physics A: Mathematical and Theoretical, **44**, 445308 (2011).
[16] M. A. Nielsen and I. L. Chuang, *Quantum Computation and Quantum Information*, 1st ed. (Cambridge University Press, 2000).
[17] J. Jin, *The Finite Element Method in Electromagnetics*, 2nd ed. (John Wiley and Sons, Inc., 2002).
[18] A. Chatterjee, J. Jin, and J. Volakis, Antennas and Propagation, IEEE Transactions on, **41**, 221 (1993).
